# Supplementary material for: Can Fair Federated Learning reduce the need for Personalisation?
Source: arXiv:2305.02728 source file (2023-05-04)
Supplement: Supplementary file 1 [file Appendix.tex]

\subsection{Full Experimental Details}\label{app:full_experimental}

\paragraph{Next-word prediction} A standard LSTM with $2$ layers, $200$ hidden units and 10 million parameters is used to predict the next word in a sentence for each client used during training or testing. We reuse the dictionary of the $50\, 000$ most frequent words compiled by \citet{yu2020salvaging}; all other words are replaced with a placeholder. The first \(90\% \) of a user's posts, chronologically, is used as a training set, with the final \(10\% \) being reserved for local testing. A separate federated testing set is maintained for evaluating global task performance during the FL training process \(\approx 5\% \) of it is used to track convergence with the full test set being used for the final evaluation after training. Federated models are trained for \(1\,000\) rounds using \(20\) clients per round rather than the \(5\,000\) rounds of \(1\,000\) clients used by \citet{yu2020salvaging}. On the client side, each model has trained for \(2\) internal epochs with a batch size of \(20\) using Stochastic Gradient Descent with the learning rate set to $40$. For adaptation, we use a learning rate of \(1\) and batch size of \(20\) for \(100\) epochs of retraining. Only \(\sim 18\,500\) clients are adapted due to resource constraints (\cref{hardware}).

\paragraph{CIFAR-10 image classification} Since CIFAR-10 is not a naturally federated dataset, a Dirichlet distribution (\(\alpha = 0.9\)) is used to simulate a Non-IID partitioning \citep{hsu2019,yu2020salvaging}. A ResNet-18 model is trained over \(1
,000\) rounds with 10 clients per round. Clients are trained using a batch size of 32 with \(2\) internal epochs and a learning rate of \(0.1\). Test accuracy is computed by multiplying a client's per-class accuracy on the CIFAR-10 test set with its proportion of the local device data. For adaptation, we use a learning rate of \(10^{-3}\) and batch size of \(32\) for \(200\) epochs of retraining. Training uses SGS with momentum $0.9$ and weight decay $0.0005$,

\paragraph{FEMNIST image classification} We use a similar experimental setup to \citet{caldas2019expanding} with a simple two-layer CNN while changing how the dataset is divided and the FL training parameters. Rather than subsampling \(5\%\) of the data, we keep the first \(350\) with more than \(10\) data points out of the total \(3\,597\) clients in the FEMINIST dataset. Since we require both local and federated testing sets, we keep \(70\%\) of a client's data for training, 10\% for local testing and add the remaining \(20\%\) to the federated test set. For the FL process, we use an aggregation learning rate of \(\eta = 1.0\) with \(10\) clients per round for \(1\,000\) rounds instead of the \(3\) clients per round used by \citet{caldas2019expanding}. We use SGD with a learning rate of \(0.1\) and a batch size of \(32\) for each client.

\subsection{Full q-FedAvg Results}\label{app:fullResults}

\begin{figure*}[!ht]
    \centering

    \includegraphics[width=\textwidth]{plots/Image_Fairplot}
    \caption[CIFAR-10 Q-FFL]{Federated performance of fair models on CIFAR-10. q-FedAvg performs marginally worse for $q \geq 10.0$, however, it must be concluded that the accuracy of the given task is not sensitive enough to fairness to draw strong conclusions.}
    \label{fig1b:globalAGGacc:FairPlot}
\end{figure*}

\begin{table}[]
    \centering
    \resizebox{\columnwidth}{!}{%
        \begin{tabular}{@{}lllllllll@{}}
            \toprule
            Objective & Adapt    & $Avg (\%)$ & $Acc < 0$ & $B 10\% (\%)$ & $W 10\% (\%)$ & $(Var_{Avg})$ & $(Var_{B})$ & $(Var_{W})$ \\ \midrule
            $q=0$     & $q=0$    & 14.185     & 53        & 20.715        & 9.392         & 13.323        & 34.379      & 20.201      \\
                      & A\_FB    & 15.87      & 0         & 25.849        & 11.311        & 29.216        & 149.736     & 3.246       \\
                      & A\_MTL   & 16.046     & 0         & 27.558        & 11.304        & 36.067        & 178.387     & 3.337       \\
                      & A\_KD    & 15.538     & 0         & 24.376        & 11.209        & 23.112        & 115.016     & 3.183       \\ \midrule
            $q=0.01$  & $q=0.01$ & 13.989     & 106       & 20.458        & 8.793         & 14.421        & 33.874      & 28.638      \\
                      & A\_FB    & 15.799     & 0         & 25.7          & 11.238        & 29.093        & 149.929     & 3.228       \\
                      & A\_MTL   & 15.833     & 1         & 27.419        & 11.057        & 36.547        & 180.574     & 3.326       \\
                      & A\_KD    & 15.495     & 0         & 24.308        & 11.175        & 23.343        & 117.768     & 3.173       \\ \midrule
            $q=0.1$   & $q=0.1$  & 14.208     & 50        & 20.907        & 9.359         & 13.742        & 35.005      & 20.733      \\
                      & A\_FB    & 15.827     & 0         & 25.964        & 11.261        & 29.505        & 149.011     & 3.212       \\
                      & A\_MTL   & 15.839     & 0         & 27.692        & 11.024        & 37.108        & 179.066     & 3.336       \\
                      & A\_KD    & 15.546     & 0         & 24.614        & 11.19         & 23.95         & 118.471     & 3.166       \\ \midrule
            $q=0.5$   & $q=0.5$  & 14.097     & 53        & 20.705        & 9.287         & 13.514        & 34.546      & 20.655      \\
                      & A\_FB    & 15.837     & 0         & 25.838        & 11.285        & 29.2          & 148.925     & 3.232       \\
                      & A\_MTL   & 15.892     & 0         & 27.555        & 11.133        & 36.531        & 179.11      & 3.26        \\
                      & A\_KD    & 15.52      & 0         & 24.42         & 11.186        & 23.402        & 116.556     & 3.199       \\ \midrule
            $q=1$     & $q=1$    & 11.397     & 70        & 17.618        & 7.047         & 12.546        & 37.951      & 19.031      \\
                      & A\_FB    & 13.463     & 0         & 22.632        & 9.256         & 25.775        & 136.853     & 1.987       \\
                      & A\_MTL   & 13.364     & 4         & 24.519        & 8.993         & 35.506        & 187.701     & 2.376       \\
                      & A\_KD    & 13.238     & 0         & 21.567        & 9.245         & 20.821        & 105.756     & 2.016       \\ \midrule
            $q=5$     & $q=5$    & 10.384     & 121       & 16.583        & 5.904         & 12.952        & 39.358      & 21.502      \\
                      & A\_FB    & 12.771     & 0         & 21.703        & 8.678         & 24.874        & 133.58      & 1.694       \\
                      & A\_MTL   & 12.838     & 6         & 23.37         & 8.548         & 33.262        & 181.204     & 2.146       \\
                      & A\_KD    & 12.492     & 0         & 20.608        & 8.614         & 19.704        & 99.431      & 1.695       \\ \midrule
        \end{tabular}
    }
    \caption{Reddit full q-FedAvg results.}
    \label{tab:res2:fed_q}
\end{table}

\begin{table}[]
    \centering
    \resizebox{\columnwidth}{!}{%
        \begin{tabular}{@{}lllllllll@{}}
            \toprule
            Objective & Adapt   & $Avg (\%)$ & $Acc < 0$ & $B 10\% (\%)$ & $W 10\% (\%)$ & $(Var_{Avg})$ & $(Var_{B})$ & $(Var_{W})$ \\ \midrule
            $q=0$     & $q=0$   & 49.652     & 0         & 56.54         & 43.045        & 15.557        & 0.79        & 2.563       \\
                      & A\_FB   & 49.669     & 0         & 56.522        & 43.145        & 15.364        & 0.839       & 2.165       \\
                      & A\_MTL  & 49.647     & 0         & 56.489        & 43.064        & 15.468        & 0.829       & 2.267       \\
                      & A\_KD   & 49.647     & 0         & 56.527        & 43.066        & 15.545        & 0.789       & 2.076       \\ \midrule
            $q=0.1$   & $q=0.1$ & 49.254     & 0         & 56.078        & 42.839        & 15.408        & 0.858       & 1.94        \\
                      & A\_FB   & 49.23      & 0         & 55.997        & 42.758        & 15.492        & 0.987       & 1.923       \\
                      & A\_MTL  & 49.257     & 0         & 55.925        & 42.933        & 15.569        & 1.129       & 2.077       \\
                      & A\_KD   & 49.248     & 0         & 56.047        & 42.82         & 15.486        & 0.996       & 1.973       \\ \midrule
            $q=1$     & $q=1$   & 49.442     & 0         & 56.297        & 42.865        & 15.614        & 1.053       & 1.991       \\
                      & A\_FB   & 49.448     & 0         & 56.308        & 42.812        & 15.729        & 0.98        & 2.423       \\
                      & A\_MTL  & 49.425     & 0         & 56.352        & 42.786        & 15.728        & 0.966       & 2.287       \\
                      & A\_KD   & 49.439     & 0         & 56.314        & 42.78         & 15.742        & 0.981       & 2.307       \\ \midrule
            $q=5$     & $q=5$   & 49.503     & 0         & 56.25         & 42.864        & 15.583        & 0.755       & 2.07        \\
                      & A\_FB   & 49.517     & 0         & 56.315        & 42.974        & 15.617        & 0.77        & 2.091       \\
                      & A\_MTL  & 49.522     & 0         & 56.404        & 42.909        & 15.651        & 0.603       & 1.874       \\
                      & A\_KD   & 49.548     & 0         & 56.416        & 42.991        & 15.531        & 0.678       & 1.902       \\ \midrule
            $q=10$    & $q=10$  & 48.286     & 0         & 54.949        & 42.033        & 14.417        & 0.608       & 1.956       \\
                      & A\_FB   & 48.3       & 0         & 54.948        & 42.096        & 14.275        & 0.424       & 1.847       \\
                      & A\_MTL  & 48.306     & 0         & 55.025        & 42.087        & 14.468        & 0.565       & 1.71        \\
                      & A\_KD   & 48.297     & 0         & 54.987        & 42.021        & 14.504        & 0.507       & 1.873       \\ \midrule
            $q=15$    & $q=15$  & 48.217     & 0         & 54.745        & 41.842        & 14.449        & 0.585       & 2.434       \\
                      & A\_FB   & 48.22      & 0         & 54.718        & 41.883        & 14.482        & 0.619       & 1.859       \\
                      & A\_MTL  & 48.202     & 0         & 54.761        & 41.824        & 14.444        & 0.614       & 2.191       \\
                      & A\_KD   & 48.193     & 0         & 54.779        & 41.713        & 14.763        & 0.564       & 2.473       \\ \bottomrule
        \end{tabular}
    }
    \caption{CIFAR-10 full q-FedAvg results.}
    \label{tab:res2b:fed_image}
\end{table}

\begin{table}[]
    \centering
    \resizebox{\columnwidth}{!}{%
        \begin{tabular}{@{}lllllllll@{}}
            \toprule
            Objective & Adapt   & $Avg (\%)$ & $Acc < 0$ & $B 10\% (\%)$ & $W 10\% (\%)$ & $(Var_{Avg})$ & $(Var_{B})$ & $(Var_{W})$ \\ \midrule
            $q=0$     & $q=0$   & 29.02      & 16        & 65.768        & 2.729         & 338.387       & 137.366     & 12.33       \\
                      & A\_FB   & 28.954     & 17        & 65.463        & 2.72          & 334.754       & 134.824     & 11.853      \\
                      & A\_MTL  & 28.994     & 16        & 65.672        & 2.802         & 336.25        & 137.507     & 11.325      \\
                      & A\_KD   & 28.986     & 16        & 65.684        & 2.788         & 337.14        & 137.796     & 11.594      \\ \midrule
            $q=0.1$   & $q=0.1$ & 27.427     & 45        & 80.262        & -23.681       & 761.163       & 117.165     & 165.003     \\
                      & A\_FB   & 26.174     & 14        & 59.483        & 2.09          & 282.14        & 128.526     & 14.212      \\
                      & A\_MTL  & 26.205     & 14        & 59.567        & 2.345         & 281.689       & 128.659     & 15.377      \\
                      & A\_KD   & 26.18      & 15        & 59.613        & 1.997         & 282.946       & 127.796     & 14.284      \\ \midrule
            $q=1$     & $q=1$   & 27.011     & 48        & 78.722        & -18.92        & 699.58        & 131.927     & 150.33      \\
                      & A\_FB   & 24.999     & 19        & 57.014        & 0.513         & 270.651       & 140.273     & 24.641      \\
                      & A\_MTL  & 25.022     & 17        & 57.179        & 0.76          & 271.681       & 136.18      & 23.188      \\
                      & A\_KD   & 25.053     & 17        & 57.165        & 0.859         & 270.926       & 135.297     & 22.658      \\ \midrule
            $q=5$     & $q=5$   & 25.048     & 46        & 73.939        & -23.702       & 683.322       & 129.091     & 177.272     \\
                      & A\_FB   & 25.385     & 18        & 56.625        & 1.758         & 264.374       & 97.084      & 8.057       \\
                      & A\_MTL  & 25.468     & 16        & 56.64         & 2.031         & 261.138       & 96.776      & 8.409       \\
                      & A\_KD   & 25.437     & 17        & 57.116        & 1.695         & 267.606       & 91.34       & 10.717      \\ \midrule
            $q=10$    & $q=10$  & 30.269     & 39        & 79.687        & -14.844       & 673.351       & 111.144     & 206.995     \\
                      & A\_FB   & 28.613     & 12        & 64.818        & 2.699         & 320.729       & 123.679     & 15.552      \\
                      & A\_MTL  & 28.612     & 14        & 64.818        & 2.516         & 321.3         & 123.679     & 15.869      \\
                      & A\_KD   & 28.563     & 14        & 64.645        & 2.52          & 320.957       & 127.618     & 15.934      \\ \midrule
            $q=15$    & $q=15$  & 23.427     & 56        & 74.969        & -23.34        & 699.404       & 145.773     & 170.676     \\
                      & A\_FB   & 22.008     & 17        & 51.138        & 1.039         & 214.214       & 115.322     & 7.717       \\
                      & A\_MTL  & 21.848     & 21        & 51.167        & 0.149         & 222.45        & 115.582     & 9.945       \\
                      & A\_KD   & 21.935     & 17        & 51.467        & 0.84          & 216.567       & 112.101     & 8.538       \\ \midrule
        \end{tabular}
    }
    \caption{FEMNIST full q-FedAvg results.}
    \label{tab:res2c:fem_fed_image}
\end{table}
